# Supplementary material for: An Efficient, Reliable and Observable Collective Communication Library in Large-scale GPU Training Clusters
Source: arXiv:2510.00991 source file (2026-06-01)
Supplement: Supplementary file 1 [file supplement.tex]

\documentclass[sigconf,10pt]{acmart}

\usepackage[english]{babel}
\usepackage{blindtext}

\usepackage[ruled,linesnumbered]{algorithm2e}
\usepackage{graphicx}
\usepackage{textcomp}
\usepackage{amsmath}
\usepackage{xcolor}
\usepackage{subfigure}
\usepackage{multirow}
\usepackage{stfloats}
\usepackage{xspace} 
\usepackage{hyperref}
\usepackage{xurl}
\usepackage{diagbox}
\usepackage{caption}
\usepackage{totpages}
\usepackage{bbding}
\usepackage{colortbl}
\usepackage{listings}
\usepackage{pifont}
\usepackage{wasysym}

\usepackage{algorithm}
\usepackage{algpseudocode}
\usepackage{hyperref}
\usepackage{xr-hyper}

\externaldocument[]{paper}
% inlined bib file
\usepackage{filecontents}

% Copyright
%\renewcommand\footnotetextcopyrightpermission[1]{} % removes footnote with conference info
\setcopyright{none}
%\setcopyright{acmcopyright}
%\setcopyright{acmlicensed}
%\setcopyright{rightsretained}
%\setcopyright{usgov}
%\setcopyright{usgovmixed}
%\setcopyright{cagov}
%\setcopyright{cagovmixed}

\settopmatter{printacmref=false, printccs=false, printfolios=true}

% DOI
\acmDOI{}

% ISBN
\acmISBN{}

%Conference
\acmConference[\scriptsize Submitted for review to EuroSys]{}
\acmYear{2027}
\copyrightyear{}

%% {} with no args suppresses printing of the price
\acmPrice{}

\begin{document}

\date{}

\newcommand\X{\textsc{VCCL}\xspace}
\newcommand\czt[1]{{\color{red}#1}}
\newcommand\zmh[1]{{\color{blue}#1}}
\newcommand\jym[1]{{\color{green}#1}}
\newcommand\zmj[1]{{\color{cyan}#1}}

\title[\scriptsize Supplemental Material – Enabling Efficient, Reliable and Observable Collective Communication in Large-scale GPU Training Clusters]{Supplemental Material – Enabling Efficient, Reliable and Observable Collective Communication in Large-scale GPU Training Clusters}

%\titlenote{Produces the permission block, and copyright information}
%\subtitle{Extended Abstract}

\author[\scriptsize Paper \#218, \ref{TotPages} pages total]{{\rm Paper \#218,  \ref{TotPages} pages total}}
%\author{Paper \# XXX, XXX pages}
% \author{Firstname Lastname}
% \authornote{Note}
% \orcid{1234-5678-9012}
% \affiliation{%
%   \institution{Affiliation}
%   \streetaddress{Address}
%   \city{City} 
%   \state{State} 
%   \postcode{Zipcode}
% }
% \email{email@domain.com}

% The default list of authors is too long for headers}
%\renewcommand{\shortauthors}{X.et al.}

%\begin{abstract}
%    \blindtext

%\end{abstract}

\maketitle

\input{texfiles/10appendix}

\bibliographystyle{ACM-Reference-Format}
\bibliography{reference}

%\bibliographystyle{ACM-Reference-Format}
%\bibliographystyle{plain}
%\bibliography{reference}

%\input{texfiles/9appendix}

%\bibliography{reference}

\end{document}
